# Supplementary material for: Liquidity Fragmentation or Optimization? Analyzing Automated Market Makers Across Ethereum and Rollups
Source: arXiv:2410.10324 source file (2025-03-12)
Supplement: Supplementary file 1 [file 99Appendix.tex]

\section{Additional Information (Section to be commented)} \label{app:1}
\paragraph{Transaction Finality}
%KG:Maybe this should be moved to the discussion part
Transaction finality refers to the period after which transaction is immutable within the blockchain ledger ledger. For L2 transactions, \emph{soft finality} indicates irreversibility from L2, whereas \emph{hard finality} - from the L1~\cite{yee2022shades} network. In the case of optimistic rollups, soft finality may last up to 7 days due to the 7-day challenge window, whereas for zk-rollups, it ranges from about an hour to a few hours depending on ZKP generations. However, with major Ethereum rollups still relying on centralized sequencers, rollup bridges provide nearly instant withdrawals from rollups, assuming trust in the operators of centralized sequencers and accommodating the finality risk.

\paragraph{Gas Fees in Rollups}
Unlike in L1 blockchains, gas fees are not known upfront for transactions in roll-ups, as it is comprised of two elements: gas fees charged by the sequencer and gas fees charged by L1 network. First, the gas fee for a transaction is estimated by the sequencer, and the address that initiated the transaction is charged the estimated gas costs. Once the transaction with a batch of other roll-up transactions is stored within the layer-1 chain, the final gas fees of L1 are known. Subsequently, the gas fee overpaid by the initial transaction originator is returned.

\paragraph{Stableswap Invariant}
        A drawback of CLMM is the necessity for LPs to continuously monitor and adjust the designated price range. The Stableswap Invariant, introduced in Curve v1 \cite{Egorov2019StableSwapLiquidity}, autonomously centralizes liquidity around the market price through the utilization of the constant \(A\). This mechanism is tailored for tokens that consistently trade at a fixed price relative to one another, such as stablecoins anchored to 1 USD. The mathematical expression of the invariant is
        \begin{equation}\label{eq:curvev1}
            K\cdot D^{N-1}\cdot \sum\limits_{i=1}^N x_i +\prod\limits_{i=1}^N x_i = K\cdot D^N + \left(\frac{D}{N} \right)^N
        \end{equation}
        with
            $$K= \frac{A\cdot\prod_{i=1}x_i}{D^N}\cdot N^N,$$
        where $A$ is a parameter.
    \paragraph{Cryptoswap Invariant}
        Curve v2 \cite{Egorov2021CurvePeg} represents a further modification of the Stableswap invariant capable of accommodating any token pairs. It employs the same mathematical formulation as equation (\ref{eq:curvev1}), with the variable $K$ being contingent upon the parameters $A$ and $\gamma$, as presented below
            \begin{equation}\label{eq:curvev2}
            K = A\cdot \underset{\text{ =: }K_0}{\underbrace{\frac{A\cdot\prod_{i=1}x_i}{D^N}\cdot N^N}} \cdot \frac{\gamma^2 }{(\gamma+1- K_0)^2}.\end{equation}
